# Supplementary material for: A Unified Approach to Enhanced Sampling
Source: arXiv:2007.03055 ancillary file (2020-08-07)
Supplement: Supplementary file 1 [file SupplementalMaterial.pdf]

# SUPPLEMENTAL MATERIAL:
# A Unified Approach to Enhanced Sampling

Michele Invernizzi,[1,2,*] Pablo M. Piaggi,[3] and Michele Parrinello[4,2,†]

[1] *Department of Physics, ETH Zurich, c/o Università della Svizzera italiana, Via Giuseppe Buffi 13, 6900 Lugano, Switzerland*

[2] *Facoltà di Informatica, Institute of Computational Science, National Center for Computational Design and Discovery of Novel Materials (MARVEL), Università della Svizzera italiana, Via Giuseppe Buffi 13, 6900 Lugano, Switzerland*

[3] *Department of Chemistry, Princeton University, Princeton, New Jersey 08540, USA*

[4] *Department of Chemistry and Applied Biosciences, ETH Zurich, c/o Università della Svizzera italiana, Via Giuseppe Buffi 13, 6900 Lugano, Switzerland, and Italian Institute of Technology, Via Morego 30, 16163 Genova, Italy*

(Dated: July 27, 2020)

## I. ALANINE DIPEPTIDE

The simulations for the alanine dipeptide example are performed with GROMACS[S1] 2018.6 patched with a custom version of PLUMED[S2] 2.6, that is available on the PLUMED-NEST website[S3]. The setup is the same of Refs. S4, S5, thus canonical ensemble (NVT) in a vacuum, Amber99-SB force field[S6], time step 2 fs, temperature $T_0 = 300$ K, velocity rescaling thermostat[S7]. The only input needed to perform the multicanonical simulation presented in the main text was the temperature range, $T_{\text{min}} = 300$ K and $T_{\text{max}} = 1000$ K, and the pace at which updating the bias potential, which was set to 500 simulation steps, thus 1 ps. For this simple system the bias converges so quickly that we did not have to drop any initial transient before performing reweighting, e.g. in producing Fig. 1 of the main text.

We show in Fig. S1 the comparison between two alanine dipeptide simulations where OPES has been used for sampling two different target distributions. On the right, Fig. S1a, we use the multicanonical expanded target presented in Sec. V A of the main text, while on the left, Fig. S1b, the well-tempered over the dihedral angles is used, with same parameters as in Ref. S5. While the two sampled ensembles are very different they can be both properly reweighted to obtain

* michele.invernizzi@phys.chem.ethz.ch

† parrinello@phys.chem.ethz.ch

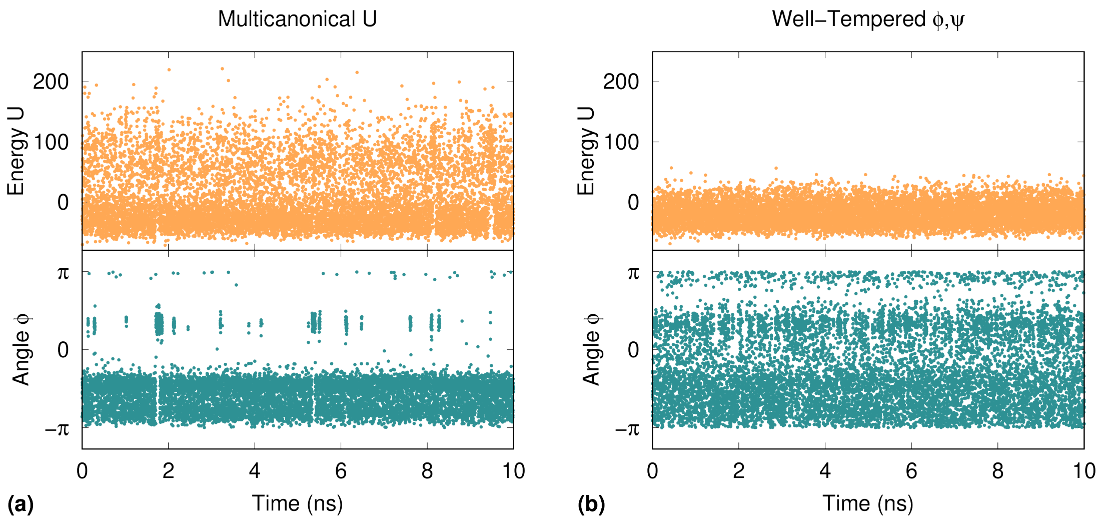


FIG. S1. Trajectories for the potential energy $U$ and the dihedral angle $\phi$ of alanine dipeptide for two different OPES run. The difference between the two is the target distribution: (a) is the multicanonical expanded one, while (b) is the well-tempered one with respect to the $\phi$ and $\psi$ angles.

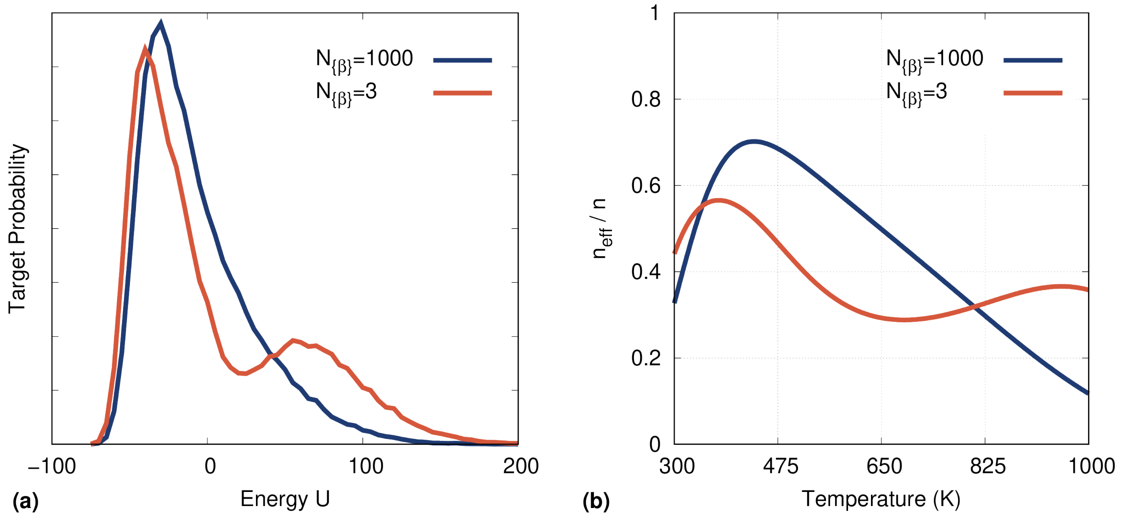


FIG. S2. Difference in using only 3 sub-temperatures, or 1000. (a) shows the energy histogram of the sampled ensemble, while (b) shows the relative effective sample size as a function of the temperature. Once the intermediate steps are enough to ensure good overlap, adding more does not lead to a better target distribution.

for instance the free energy difference between the two metastable $\Delta F_{AB}$ at 300 K. While for calculating $\Delta F_{AB}$ it is more convenient to directly bias $\phi$ and $\psi$, this requires some knowledge of the system, and in general it is far from trivial to identify good CVs, thus a more generic approach such as the multicanonical one can be useful.

Next in Fig. S2 we show how the multicanonical target distribution for alanine dipeptide changes

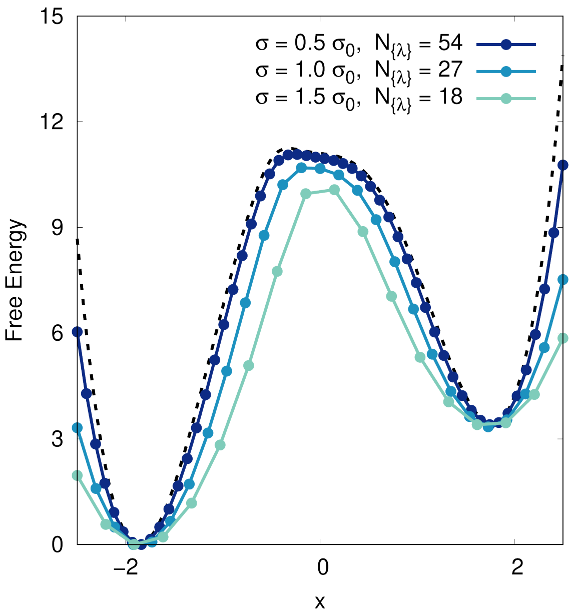


FIG. S3. The $\Delta F(x_\lambda)$ of the double-well model, for different choices of $\sigma$. The black dotted line is the reference free energy surface. The case $\sigma = 0.1\,\sigma_0$, $N_{\{\lambda\}} = 270$, is not shown because it perfectly matches the reference line.

when varying the number $N_{\{\beta\}}$ of intermediate temperatures. By default the number of intermediate temperatures is determined automatically via a short (100 ps in this case) unbiased simulation (see Sec. V). In the considered alanine example this suggest the use of just 3 temperatures, equispaced in $\beta$: $T_1 = 300$ K, $T_2 = 461.538$ K, $T_3 = 1000$ K. As discussed in Sec. VII of the main text adding more intermediate temperatures might not bring better sampling. We can see this by plotting the effective sample size $n_{\text{eff}}$ relative to the total sample size $n$. We see that by using $N_{\{\beta\}} = 3$ we can cover in a more uniform way the temperature interval, compared to the case of $N_{\{\beta\}} = 100$. This suggest that the optimal target distribution is not the one obtained by substituting the sum with an integral.

## II. DOUBLE-WELL MODEL

The double-well Langevin model is the same use in Refs. S4, S5, and is implemented in PLUMED. The 2D potential energy is defined by rotating of an angle $\theta = -0.6\frac{\pi}{4}$ the following potential:

$$u(x, y) = x^4 + y^4 - 2\,x^2 - 4\,y^2 + xy + 0.3\,x + 0.1\,y\,. \tag{S1}$$

Fig. S3 shows how the estimated $\Delta F(x_\lambda)$ changes when varying the width of the umbrellas $\sigma$.

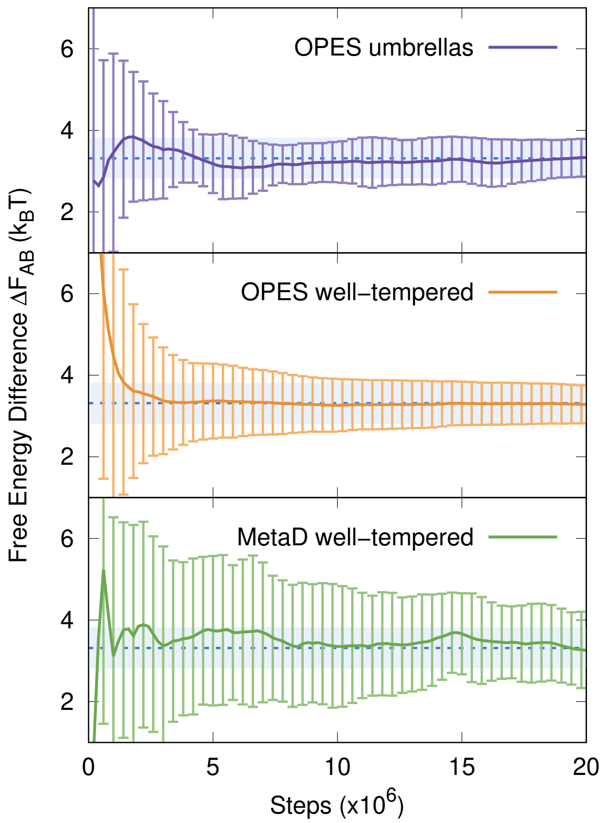


FIG. S4. The estimate of the free energy difference $\Delta F_{AB}$ between the two basins of the model, obtained with different methods, by averaging 10 independent runs. The run obtained using OPES with the multiumbrella target uses $\sigma = \sigma_0 = 0.185815$. The results for OPES with a well-tempered target and metadynamics are taken from Ref. [S5].

The corresponding target distribution along $x$ are shown in Fig. 4b of the main text. The estimate of the free energy surface $F(x)$ obtained from reweighting is instead independent from the choice of $\sigma$.

Fig. S4 presents a comparison between OPES using different kind of target distributions, namely the multiumbrella one and the well-tempered one, and metadynamics. In a one dimensional problem the multiumbrellas target can be slightly more efficient than the well-tempered one. However, OPES with a well-tempered target is more versatile, since it can be used also without knowing in advance the CV range, and can be scaled up to higher dimensions more efficiently, as shown in Ref. [S5].

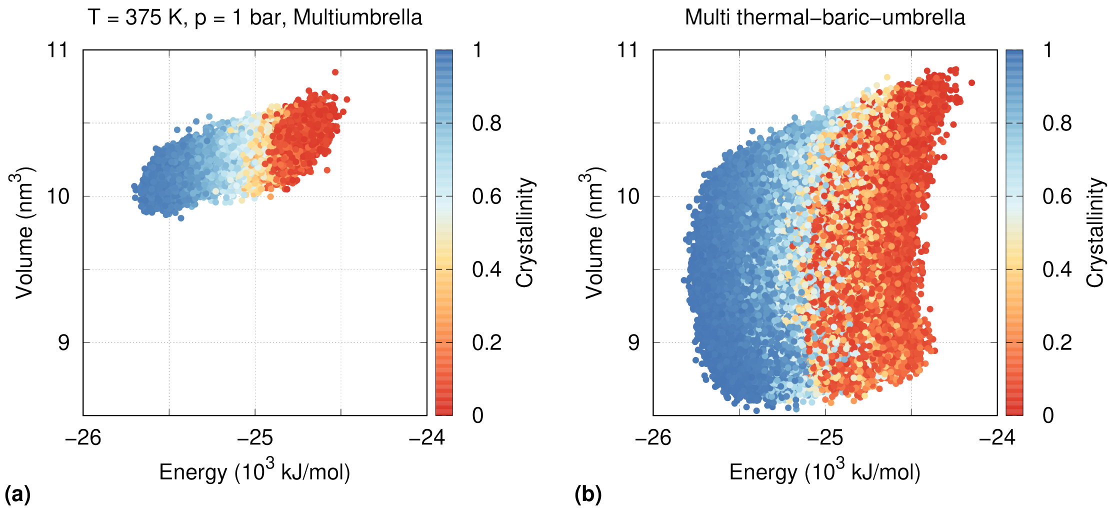


FIG. S5. Sampled sodium configurations in the energy-volume space, (a) at fixed temperature and pressure, biasing the crystallinity CV with a multiumbrella target, and (b) multithermal, multibaric, and multiumbrella simulation, the same used for Fig. 5 in the main text.

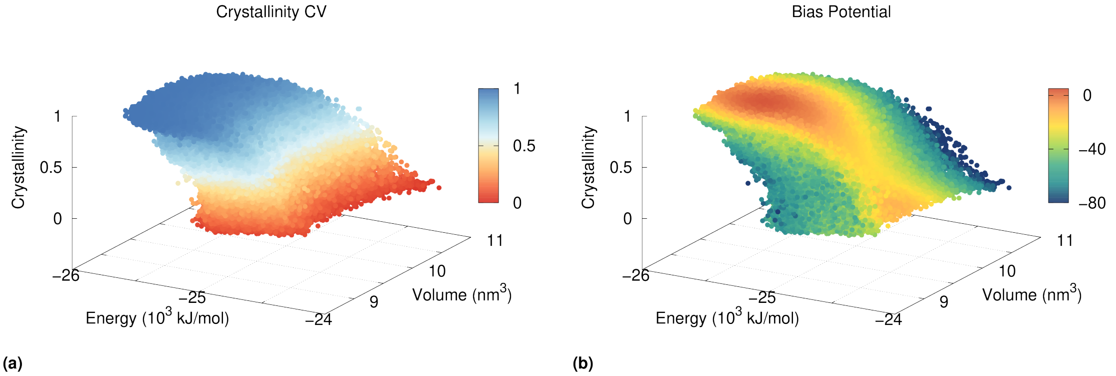


FIG. S6. Sampled sodium configurations for the multithermal-multibaric-multiumbrella simulation in the energy-volume-crystallinity space. (a) Colored accordingly to the crystallinity CV $s$. (b) Colored accordingly to the value of the bias $v(U, V, s)$. The hourglass shape described in Ref. S8 is clearly visible.

## III. SODIUM

The sodium simulations were performed in the same setting as Ref. [S8]. We show the sampled space in Figs. S5 and S6.

---

[S1] M. J. Abraham, T. Murtola, R. Schulz, S. Páll, J. C. Smith, B. Hess, and E. Lindahl, GROMACS: High performance molecular simulations through multi-level parallelism from laptops to supercomputers,

SoftwareX **1-2**, 19 (2015).

[S2] G. A. Tribello, M. Bonomi, D. Branduardi, C. Camilloni, and G. Bussi, PLUMED 2: New feathers for an old bird, Computer Physics Communications **185**, 604 (2014).

[S3] The PLUMED consortium, Promoting transparency and reproducibility in enhanced molecular simulations, Nature Methods **16**, 670 (2019).

[S4] M. Invernizzi and M. Parrinello, Making the Best of a Bad Situation: A Multiscale Approach to Free Energy Calculation, Journal of Chemical Theory and Computation **15**, 2187 (2019).

[S5] M. Invernizzi and M. Parrinello, Rethinking Metadynamics: From Bias Potentials to Probability Distributions, The Journal of Physical Chemistry Letters **11**, 2731 (2020), arXiv:1909.07250.

[S6] V. Hornak, R. Abel, A. Okur, B. Strockbine, A. Roitberg, and C. Simmerling, Comparison of multiple Amber force fields and development of improved protein backbone parameters, Proteins: Structure, Function, and Bioinformatics **65**, 712 (2006).

[S7] G. Bussi, D. Donadio, and M. Parrinello, Canonical sampling through velocity rescaling, The Journal of Chemical Physics **126**, 014101 (2007), arXiv:0803.4060.

[S8] P. M. Piaggi and M. Parrinello, Calculation of phase diagrams in the multithermal-multibaric ensemble, The Journal of Chemical Physics **150**, 244119 (2019).
